# Supplementary material for: Towards Stochastic Fault-tolerant Control using Precision Learning and Active Inference
Source: arXiv:2109.05870 source file (2021-09-13)
Supplement: Supplementary file 1 [file appendix.tex]

\section{Appendix: Deterministic fault detection, isolation, and recovery}
\label{sec:hard_update_deterministic}
In this section we describe how the sensory prediction errors can be used as residual signals to be monitored and how to perform fault detection and isolation. Without loss of generality, for these derivations we will consider only the proprioceptive sensors and we discretize the continuous dynamics with first order Euler integration. First of all, according to the approximated system's dynamics in equation \eqref{eq:euler_integration_a}, and expanding the second term in equation \eqref{eq:u-AIC_F_minimize_a} where $F$ is computed as in equation \eqref{eq:laplace_F_final_vector}, the state estimation law can be rewritten as:
\begin{equation}
\label{eq:estimator_mu}
\bm \mu_{k+1} = \gamma (\bm \mu_k, \bm u_k) + \Lambda(\bm g(\bm\mu_k) - \bm y_k)\\
\end{equation}

Equation \eqref{eq:estimator_mu} represents the dynamics of an estimator where stability results from the value that we obtain for diagonal matrix $\Lambda$. For the sake of brevity, the algebraic manipulations leading to eq.~\eqref{eq:estimator_mu} are not reported here. Anyway, it is important to 
note that $\gamma$ and $\Lambda$ are known expressions resulting from the partial derivatives of $F$. Furthermore, in \cite{meera_colored_noise} it has been shown how the free-energy principle can be used to derive stable state observers, for a linear case with coloured noise. The term $(\bm y_k - \bm g(\bm\mu_k))$ represents the sensory prediction errors. 

In the d-AIC system's dynamics can be represented in general as (see \cite{baioumy2021ECC}):

\begin{equation}
\label{eq:dynamics_x}
\begin{cases}
\bm x_{k+1} = \gamma (\bm x_k, \bm u_k) + \phi(\bm x_k, \bm u_k, \bm \rho_k)\\
\bm y_k = \bm x_k + \bm z_k
\end{cases}
\end{equation}

where $\bm x_k\in\mathbb{R}^n$ and  $\bm u_k\in\mathbb{R}^m$ are the state and input variables, while $\gamma (\bm x_k, \bm u_k):\mathbb{R}^n\times\mathbb{R}^m \mapsto \mathbb{R}^n$ represents the dynamics of the system in healthy conditions. $\bm y_k\in\mathbb{R}^n$ is the measurement of the full state which is affected by the presence of measurement noise $\bm z_k\in\mathbb{R}^n$.
The expressions obtained so far for the system dynamics will allow us to cast easily a model-based fault diagnosis approach in the current framework, even if the knowledge of an a-priori model is not needed.

The real system can be affected by faults which are represented by the fault function $\phi(\bm x_k, \bm u_k, \bm \rho_k):\mathbb{R}^n\times\mathbb{R}^m\times \mathbb{R}^l\mapsto \mathbb{R}^n$.  The unknown parameter $\bm \rho_k$ determines the fault amplitude and shall be such that $\phi(\bm x_k, \bm u_k, \bm 0) = 0$. 

\subsection{Residual generation}
We define the residuals for fault detection as the sensory prediction errors $\bm r_{k} = \bm y_k - \bm g(\bm\mu_k)$. Thus, according to \eqref{eq:dynamics_x}, \eqref{eq:estimator_mu} and following \cite{Rostampour2017,Rostampour2018}, the residuals dynamics will be given by:
\begin{equation}
\label{eq:rk+1}
    \bm r_{k+1} = \Lambda\bm r_k + \bm \delta_k + \phi(\bm x_k, \bm u_k, \bm \rho_k) 
\end{equation}
where:
\begin{equation}
    \bm \delta_k = \gamma (\bm y_k - \bm z_k, \bm u_k) - \gamma (\bm \mu_k, \bm u_k) + \bm z_{k+1}
\end{equation}

The stochastic process $\bm \delta_k$, is the random total uncertainty which affects the residuals generation. It follows that $\bm \delta_k$ is in the probability space ($\Delta_k, \mathcal{B}(\Delta_k), \mathbf{P}_{\bm \delta_k}$) where $\Delta_k$ is obtained by letting $\bm z_k$ and $\bm z_{k+1}$ vary over $\mathcal{Z}$. Apart from simple cases, it is not possible to obtain a closed form for this set, thus numerical approximations are used instead. 

The residual $\bm r_{k+1}$ can be seen as a random variable in the same probability space of $\bm \delta_k$ \cite{Rostampour2017}. 

% \begin{figure}[!htb]
%     \centering
%     \includegraphics[width=0.9\linewidth]{images/residualset.pdf}
%     \caption{Healthy residual set at time $k+1$ as image obtained from the output of \eqref{eq:rk+1}.}
%     \label{fig:residualset}
% \end{figure}

% The residual set $\mathcal{R}_{k+1}$ at the next time step $k+1$ can be seen as the image obtained by computing the output of \eqref{eq:rk+1}, where the total uncertainty $\bm \delta_k$ varies over its domain $\Delta_k$. Note that the healthy residuals can be characterized by setting $\bm \rho_k = 0$. 

% \begin{rem}
% While the system dynamics $\gamma$ and the fault function $\phi$ have been introduced for analysis purposes, they do not correspond to known models of the healthy and faulty behaviours. In particular, $\gamma$ is obtained via algebraic manipulations from current free energy framework's update equations. In particular, the residual $r$ for implementing the detection and isolation logic described next can be directly computed from the current belief and measurement. Indeed, the proposed fault diagnosis approach based on the d-AIC is completely model-free.
% \end{rem}

\subsection{Threshold for fault detection}
\label{sec:FD}
The threshold for fault detection using the residuals just defined, can be computed in several ways. One could collect a set of residuals during healthy operations and then compute the sufficient statistics to derive a static threshold to use at run-time \cite{kumar2009approach}. Deterministic thresholds of this kind, however, are overly conservative. As in \cite{Rostampour2018}, we consider a probabilistically robust detection logic of the form:
\begin{equation}
    \label{eq:detection}
    d_M(\bm r_{k+1})\leq \frac{n}{\alpha}  \triangleq \overline{d_M}
\end{equation}
where $\tau$ is the detection threshold and $d_M(\cdot)$ indicates the Mahalanobis distance of the residuals. $d_M$ is defined as
\begin{equation}
    d_M(\bm r) = \sqrt{(\bm r-\bar{\bm r})^\top C_r^{-1}(\bm r-\bar{\bm r})} 
\end{equation}
where $\bar{\bm r} \triangleq \mathbb{E}[\bm r]\in \mathbb{R}^n$ and $C_r \triangleq Cov[\bm r] \in \mathbb{R}^{n\times n}$ are the expected value and covariance matrix of the residuals. According to the Multivariate Chebyshev Inequality \cite{chen2007new}, it holds:
\begin{equation} 
    Pr[ d_M(\bm r_k) \geq \frac{n}{\alpha}] \leq \alpha,\hspace{5mm} \forall \alpha \in [0, \, 1 ]
\end{equation}
This means that, in healthy conditions, the probability of a false alarm, that is $d_M$ exceeding the threshold $\bar d_M$, is upper bounded by $\alpha$.
The value $\alpha$ can be tuned to achieve the desired probabilistic robustness of the threshold. 
% The present detection logic is equivalent to check if the residual at time step $k+1$ belongs to a time varying ellipsoid with it's center at the mean $\bar{\bm r}_{k+1}$ and covariance $C_{r_{k+1}}$. 

% It is a bit of a stretch to say that an ellipsoid has a mean and a covariance. The centre of it is equal to the mean, its axes lay parallel to the eigenvectors of C, and the length of the axes is proportional to the eigenvalues of C

In the general nonlinear case, these moments can be approximated by their sampled counterparts obtained in healthy conditions. 

\subsection{Fault isolation}
The detection policy in equation \eqref{eq:detection} results effective to label the system as healthy or faulty. However, it is not possible to use the same SPE generated through equation \eqref{eq:laplace_F_final_vector} for fault isolation. In fact, the free-energy is computed as a weighted sum of the squared prediction errors fusing different sensory sources. It is clear that if one of the sources is faulty, the overall state estimation and control will be affected. This means that when a fault occurs, its effects will propagate to all the SPE in equation \eqref{eq:laplace_F_final_vector}. 
To solve this problem, we define $F_p$ which only accounts for the prediction errors $\bm{\varepsilon}_{y_q}$, $\bm{\varepsilon}_{y_{\dot{q}}}$ and $F_v$ which accounts for $\bm{\varepsilon}_{y_v}$. Doing so, we can isolate encoder and camera faults since state estimation is now done using two independent measurement sources. Note that $F_p$ and $F_v$ are only used for fault isolation and not for control. 

\subsection{Fault recovery}
Once a fault is detected and isolated, fault recovery is triggered. To do so, we exploit the fact that the controller encodes the precision matrices (inverse covariance) $P_{y_q}$, $P_{y_{\dot{q}}}$ and $P_{y_v}$ to define the confidence about each sensory input. Every sensor contributes to the posterior prediction of the most plausible state of the robot arm. If a sensor is marked as faulty, it is sufficient to set its corresponding precision matrix to zero. The controller can thus exploit the sensory redundancy for two reasons: to have a better a posteriori approximation of the states, and to compensate for missing or wrong sensory data. Once a fault is detected and isolated, the precision matrix of the faulty sensor $P_{fs}$ is reduced to zero:
\begin{equation}
    P_{fs} = \bm 0
\end{equation}

% Interestingly, the active inference framework allows also for hyper-parameters (precision) learning \cite{baioumy2020active, tutorial} 
% This was not possible with the standard formulation of the AIC, since biased state estimation hindered hyper-parameters learning for fault recovery purposes. Learning the precision matrices associated with sensory readings is out of the scope of this work, but will be thoroughly investigated in the future. 
